# Supplementary material for: Experimental demonstration of kinetic proofreading inherited in ligation-based information replication
Source: arXiv:2505.08232 source file (2025-10-24)
Supplement: Supplementary file 1 [file SI.pdf]

# Supplemental Material for "Experimental demonstration of kinetic proofreading inherited in ligation-based information replication"

Hiroyuki Aoyanagi,[1] Yasuhiro Magi,[1] and Shoichi Toyabe[1,*]
[1] *Department of Applied Physics, Graduate School of Engineering, Tohoku University, Sendai, Japan*
(Dated: May 13, 2025)

## S1. EXPERIMENT

### S1.1. DNA sequences

DNA oligonucleotides with either a reverse-phase cartridge or PAGE purification grade were purchased from IDT or Eurofins Genomics (see Table S1 for the sequences). Substrates B, B', C-X, BC-X, and B'C-Y were phosphorylated. The template $\overline{\mathrm{ABC}}$ (written from 3' to 5' ends) consists of 74 bases, consisting of three 20-base domains for substrate hybridization and 7-base overhangs at both ends. These 7-base overhangs are essential for distinguishing the template DNA from the products in PAGE analysis.The substrates used were U-A, B, B', and C-X for the middle error case and U-A, U'-A', B, and C-X for the terminal error case. The sequence A' and B' contains a two-base mutation relative to substrate A and B, respectively. Tag sequences U, U', X, and Y correspond to primer-binding regions used in the quantitative PCR (qPCR) experiments. The qPCR protocol is described in Section S1.4.

TABLE S1. The DNA sequences used in the ligation experiment. PHO indicates phosphate group.

| Name | Sequence ($5' \to 3'$) |
|---|---|
| $\overline{\mathrm{ABC}}$ | gtgaatt aaccaggaagtgagacgaa<br>taacgtaggtgttggctcta tatccatcacgactcagcaaa tgtactg |
| U-A | aata gcataccgatgcttgaccacat attgctgagtcgtgatggat |
| U'-A' | aata gcataccgatgcttgaccacgc attgctgggtcgcgatggat |
| B | [PHO]-atagagccaacacctacgtt |
| B' | [PHO]-atagagctaacatctacgtt |
| C-X | [PHO]-attcgtctcacttcctggtt tcggacagtctgctacagcg |
| BC-X | [PHO]-atagagccaacacctacgtt attcgtctcacttcctggtt tcggacagtctgctacagcg |
| B'C-Y | [PHO]-atagagctaacatctacgtt attcgtctcacttcctggtt tacacatgacgcacggatgc |
| U-AB | gcataccgatgcttgaccacat attgctgagtcgtgatggat atagagccaacacctacgtt |
| U'-A'B | gcataccgatgcttgaccacgc attgctgggtcgcgatggat atagagccaacacctacgtt |

### S1.2. Ligation reaction

The reaction mixture had a total volume of 20 µL, containing 640 units/mL of thermostable Taq DNA ligase (New England Biolabs, MA, USA), 1× Taq DNA Ligase Buffer, 5 nM of the template $\overline{\mathrm{ABC}}$, and each substrates at the total substrate concentration of 200 nM. When A and A' or B and B' are mixed, each substrate was added at a concentration of 100 nM so that $[\mathrm{A}] + [\mathrm{A}'] = 200\,\mathrm{nM}$ or $[\mathrm{B}] + [\mathrm{B}'] = 200\,\mathrm{nM}$. The thermal cycling protocol started with a 5 s denaturation step at 90 °C, followed by 20 s incubation steps at five different temperatures: 64.8, 66.0, 66.6, 68.7, and 70.5 °C. After the thermal cycling, an equal volume of loading buffer, consisting of 10 M urea and 240 mM ethylenediaminetetraacetic acid (EDTA) dissolved in 1× Tris-borate-EDTA buffer (TBE buffer), was added so as to stop the reaction.

* toyabe@tohoku.ac.jp

### S1.3. Measurement of product amount by polyacrylamide gel electrophoresis

Following the thermal cycling, we quantified the amount of product using denaturing polyacrylamide gel electrophoresis (PAGE). To ensure complete denaturation of the products from the template strand, PAGE was performed at 70 °C by immersing the chamber in a thermostatic incubator with a constant voltage of 200 V. Alongside the experimental samples, reference DNA strands of various lengths and concentrations were loaded in separate lanes. The gel was stained with 1× SYBR Gold (Thermo Fisher Scientific) dissolved in 1× TBE buffer. Gel images were captured using a 16-bit scanner (LI-COR) [Fig. S1a].

The gel images were processed and analyzed using a lab-developed Python program using the OpenCV library. Each lane was cropped into a rectangular region, and the fluorescence intensity of each pixel was averaged along the direction orthogonal to the lane. This yielded a one-dimensional intensity profile for each lane [Fig. S1b]. To remove background noise, we applied the rolling minimum method [1] and subtracted the resulting background signal from the raw intensity data. The remaining signal peaks, corresponding to DNA products, were fitted using a Gaussian mixture model. Peak fitting was performed with the minimize function from the SciPy library, and the intensity of each peak was quantified as the area under the corresponding Gaussian curve.

The fluorescence intensity is approximately proportional to the molecular weight and DNA concentration. We first constructed a calibration curve that relates fluorescence intensity to DNA mass. The DNA mass $w$ in each reference band was calculated using the following equation:

$$w = cVMd, \tag{S1}$$

where $c$ is the molar concentration of the reference DNA, $V$ is the sample volume loaded into the gel, $M$ is the molecular weight, and $d$ is the dilution factor. The measured intensity-mass relations were fitted with a linear function under a constraint of zero intercept [Fig. S1c]. Product concentrations were estimated based on this calibration curve. Because background levels and gel staining can vary between experiments, calibration curves were produced for each gel.

After imaging the gel, DNA was extracted from each product band. The gel around a target band was excised and transferred into microtubes (LDNA LoBind, Eppendorf) and crushed. We poured pure water to the microtube and incubated it at 37 °C for 1 hour in a thermostatic shaking incubator. The supernatant was collected and used for qPCR measurement [Section S1.4].

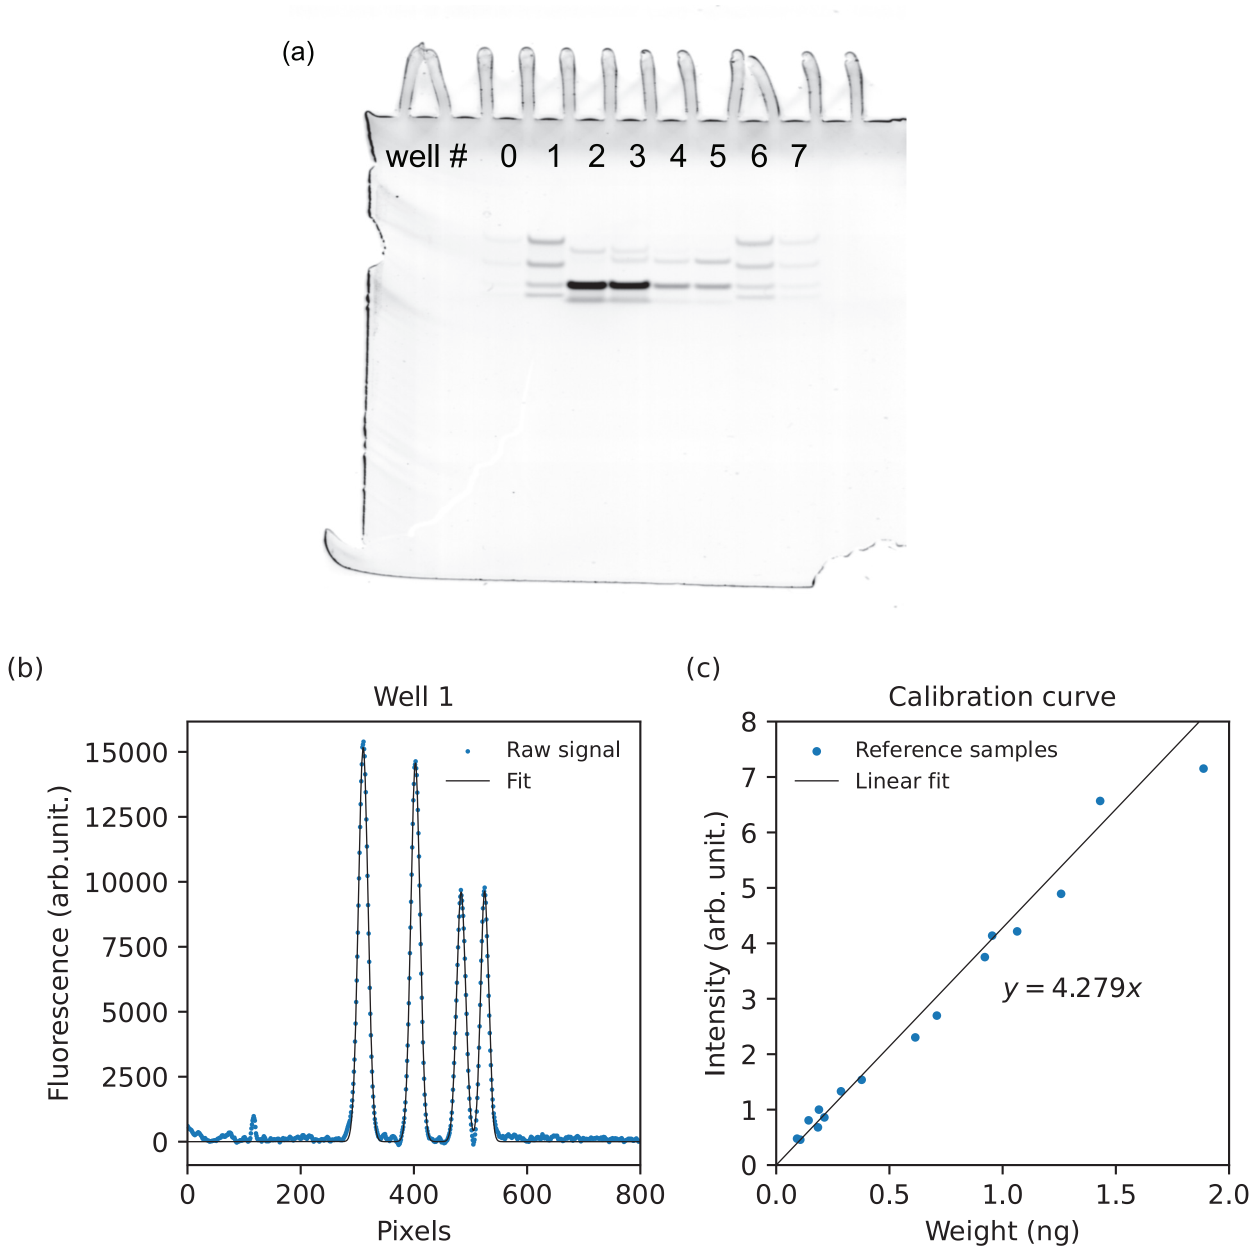


FIG. S1. (a) An example of the gel picture. Two lanes on each side correspond to the reference DNA. (b) Intensity profile of well 1 of the gel in (a) after subtracting the background signal. Scatters correspond to the raw data, and the line corresponds to the fitted result by the Gaussian mixture. (c) Calibration curve. For each reference lane (wells 0, 1, 6, and 7), we extracted the 1D fluorescence profile as in (b) and calculated the area under each Gaussian peak. Fluorescence intensities were then associated with the known DNA weights. Dots represent reference data points, and the line indicates the linear fit.

### S1.4. Measurement of error fraction by quantitative PCR

Assuming that the concentration ratio between the correct and wrong products in the supernatant remained unchanged from the original sample prior to PAGE, we quantified the error fraction using the supernatant obtained from the DNA extraction step by quantitative PCR (qPCR). The qPCR reaction mixture contains the supernatant, 200 nM of each primer [Table S2], and Luna Universal qPCR Master Mix (New England Biolabs). The thermal cycling protocol consists of an initial denaturation step at 95 °C for 10 s, followed by an annealing step at either 65 °C or 50 °C for 20 s, and an extension step at 72 °C for 5 s. qPCR was performed on a CFX96 Touch Real-Time PCR cycler (Bio-Rad). The fluorescence data were analyzed to determine the Ct values by the method described in [2]. For each experimental condition, we prepared independent calibration curves. The sequences of the DNA templates used to construct the calibration curves are listed in Table S3. To establish the relationship between Ct values and template concentrations, we performed serial dilutions of the template strand solution with a ratio of 1/8 and measured the corresponding Ct values. The combinations of primer sets and template strands used are summarized in Table S4.

The qPCR data were fitted using the following equation:

$$\mathrm{Ct} = -a \log_8 [C] + b \tag{S2}$$

where Ct represents the threshold cycle of amplification, $C$ is the template concentration, $a$ is the slope, and $b$ is the $y$-intercept. See Fig. S2 and Table S4 for the results.

TABLE S2. The DNA sequences of primer sequences

| Name | Sequence ($5' \to 3'$) |
|---|---|
| p-U | gcataccgatgcttgaccacat |
| p-U’ | gcataccgatgcttgaccacgc |
| p-X | cgctgtagcagactgtccga |
| p-Y | gcatccgtgcgtcatgtgta |
| p-ABC | ggaagtg agacg aattt cgtagg tgttg |
| p-AB’C | ggaagtg agacg aattt cgtaga tgtta |
| p-BCX | atggatttagagccaacac |
| p-B’CX | tgagtcgtgatggat taagagctaacat |
| p-B | atagagccaacacctacgt |

TABLE S3. The DNA sequences of the template for the calibration curve measurement

| Name | Sequence ($5' \to 3'$) |
|---|---|
| t-U-X | gcataccgatgcttgaccacat attgctgagt cttcctggtt tcggacagtctgctacagcg |
| t-trimer(B’) | gcataccgatgcttgaccacat attgctgagtcgtgatggat atagagctaacatctacgtt attcgtctcacttcctggtt |
| t-trimer(A’) | gcataccgatgcttgaccacgc attgctgggt cttcctggtt tcggacagtctgctacagcg |
| t-U-Y | gcataccgatgcttgaccacat attgctgagt cttcctggtt tacacatgacgcacggatgc |
| t-UAB | gcataccgatgcttgaccacat attgctgagtcgtgatggat atagagccaacacctacgtt |
| t-UAB’ | gcataccgatgcttgaccacat attgctgagtcgtgatggat atagagctaacatctacgtt |
| t-BCX | atagagccaacacctacgttattcgtctcacttcctggtttcggacagtctgctacagcg |
| t-B’CX | atagagctaacatctacgttattcgtctcacttcctggtttcggacagtctgctacagcg |
| t-U’A’B | gcataccgatgcttgaccacgc attgctgggtcgcgatggat atagagccaacacctacgtt |

TABLE S4. The combinations of the primer set and the template for the calibration with the obtained calibration parameters.

| Products | Forward primer | Reverse primer | Templates | Annealing temp. (°C) | $a$ | $b$ |
|---|---|---|---|---|---|---|
| UABCX+UAB'CX | p-U | p-X | t-U-X | 65 | -2.87 | 15.9 |
| UAB'CX | p-U | p-AB'C | t-trimer(B') | 65 | -3.06 | 18.5 |
| U'A'BCX | p-U' | p-X | t-trimer(A') | 65 | -2.93 | 17.2 |
| UABCY | p-U | p-Y | t-U-Y | 65 | -3.00 | 17.4 |
| UAB | p-U | p-ABC | t-UAB | 50 | -2.92 | 19.2 |
| UAB' | p-U | p-AB'C | t-UAB' | 50 | -3.08 | 24.5 |
| UAB | p-U | p-B | t-UAB | 65 | -2.88 | 16.9 |
| U'A'B | p-U' | p-B | t-U'A'B | 65 | -2.89 | 16.9 |
| BCX | p-BCX | p-X | t-BCX | 50 | -3.09 | 17.1 |
| B'CX | p-B'CX | p-X | t-B'CX | 50 | -3.31 | 22.4 |

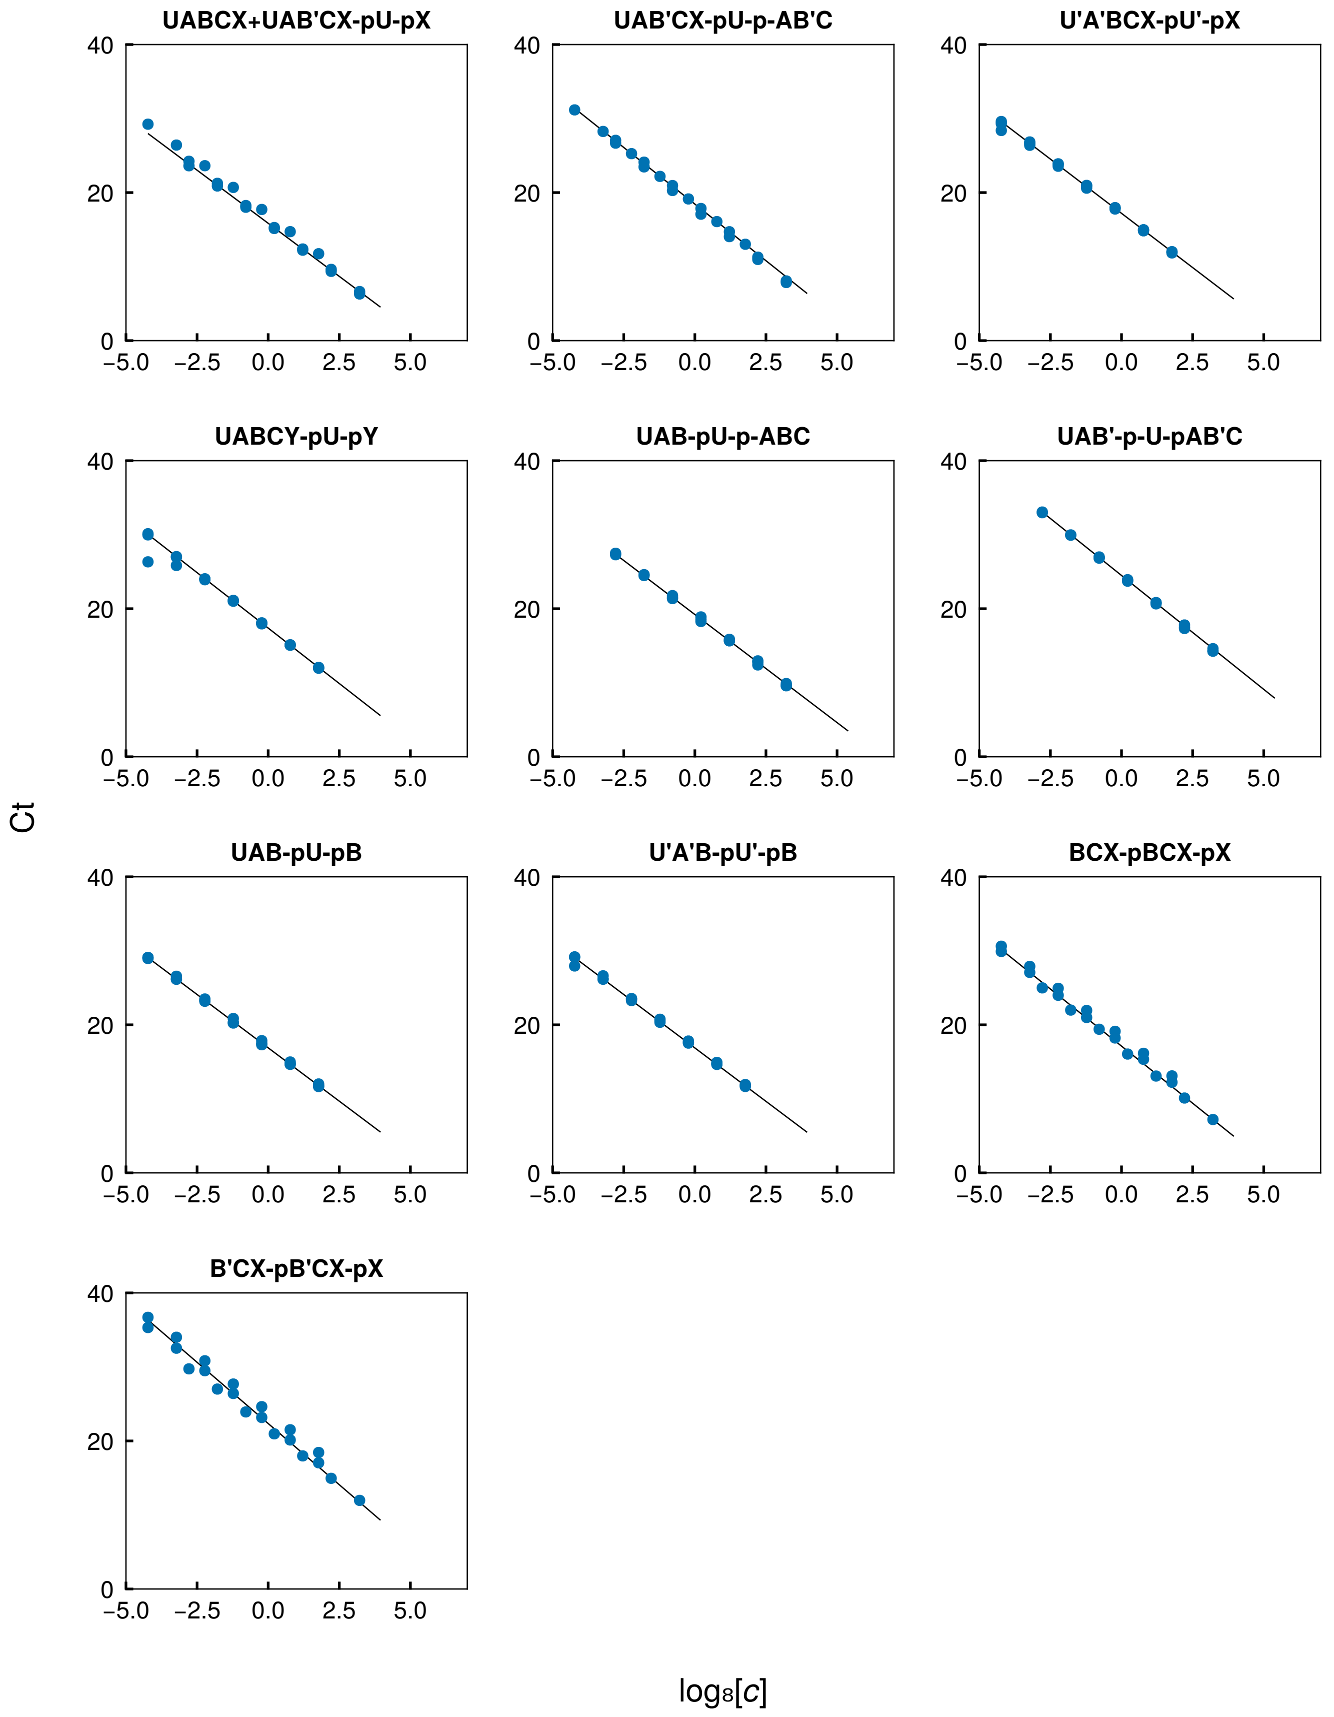


FIG. S2. Calibration curves used for quantifying the error fraction.

## S1.5. Melting curve experiment

The melting curve experiment was conducted to determine the thermodynamic parameters of DNA hybridization. The temperature was gradually decreased from 90 °C to 30 °C with −0.2 °C steps, allowing for controlled denaturation and annealing of the DNA strands. Fluorescence intensity was measured at each temperature step. Each sample was prepared with a DNA concentration of 100 nM, and SYBR Green I fluorescent dye was added at 0.25× concentration to monitor melting behavior via fluorescence. To prevent nonspecific hybridizations, the tag sequences were not used for the monomer strands [Table S5]. Reactions were carried out in 1× Taq DNA Ligase Reaction Buffer (New England Biolabs), consistent with the conditions used in the main experiments. The resulting fluorescence data were analyzed to extract thermodynamic parameters, following the methodology described in our previous work [3], which is briefly outlined below.

TABLE S5. The DNA sequences used for the melting curve experiment.

| Name | Sequence ($5' \to 3'$) |
|---|---|
| $\overline{\text{A}}$ | tatccatcacgactcagcaa |
| $\overline{\text{B}}$ | taacgtaggtgttggctcta |
| $\overline{\text{C}}$ | taaccaggaagtgagacgaat |
| $\overline{\text{AB}}$ | taacgtaggtgttggctcta tatccatcacgactcagcaa |
| $\overline{\text{BC}}$ | taaccaggaagtgagacgaa taacgtaggtgttggctctat |
| A | attgctgagtcgtgatggat |
| B | [PHO]atagagccaacacctacgtt |
| B' | [PHO]atagagctaacatctacgtt |
| C | attcgtctcacttcctggtt |
| UAB | gcataccgatgcttgaccacat attgctgagtcgtgatggat atagagccaacacctacgtt |
| UAB' | gcataccgatgcttgaccacat attgctgagtcgtgatggat atagagctaacatctacgtt |
| BCX | atagagccaacacctacgtt attcgtctcacttcctggtt tcggacagtctgctacagcg |
| B'CX | atagagctaacatctacgtt attcgtctcacttcctggtt tcggacagtctgctacagcg |

The standard free energy change, $\Delta G^\circ(T)$, was estimated from fluorescence intensity data by using the exponential background subtraction method [4]. Assuming that the normalized fluorescence signal $\alpha$ corresponds to the fraction of double-stranded DNA (dsDNA), $\Delta G^\circ(T)$ was calculated as

$$\Delta G^\circ(T) = k_{\mathrm{B}} T \ln \left[ \frac{C_0 (1-\alpha)^2}{\alpha} \right], \tag{S3}$$

where $C_0 = 100$ nM is the concentration of each DNA strand, $k_{\mathrm{B}}$ is the Boltzmann constant, and $T$ is the absolute temperature. The temperature dependence of $\Delta G^\circ$ was then fitted with a linear function to determine the standard enthalpy $\Delta H^\circ$ and the standard entropy $\Delta S^\circ$ using the relation:

$$\Delta G^\circ(T) = \Delta H^\circ - T \Delta S^\circ, \tag{S4}$$

assuming that both $\Delta H^\circ$ and $\Delta S^\circ$ are independent of $T$. Using the fitted parameters, the dissociation constant $K_{\mathrm{d}}$ was calculated as

$$K_{\mathrm{d}} = \frac{k_{\mathrm{off}}}{k_{\mathrm{on}}} = \exp\left( \frac{\Delta G^\circ(T)}{k_{\mathrm{B}} T} \right). \tag{S5}$$

The resulting thermodynamic profiles are shown in Fig. S3, and the obtained values are summarized in Table S6.

By plotting each $\Delta H^\circ$ and $\Delta S^\circ$ value against the strand length $i$, we observed clear linear trends for both correct and wrong substrates. To quantify these trend, we fitted the data using the following equations:

$$\Delta H^\circ_{\mathrm{R/W}} = \phi_{\Delta H^\circ} \cdot i + \psi_{\Delta H^\circ,\mathrm{R/W}}, \tag{S6}$$

$$\Delta S^\circ_{\mathrm{R/W}} = \phi_{\Delta S^\circ} \cdot i + \psi_{\Delta S^\circ,\mathrm{R/W}}, \tag{S7}$$

where $\phi$ and $\psi$ represent the slope and intercept for each thermodynamic parameter, respectively. The subscripts R and W refer to correct and wrong monomers. In this model, the slope values $\phi_{\Delta H^\circ}$ and $\phi_{\Delta S^\circ}$ are common between the correct and wrong monomers, representing the average stabilization per additional nucleotide. The differences in intercepts $\psi_{\Delta H^\circ,\mathrm{W}} - \psi_{\Delta H^\circ,\mathrm{R}}$ and $\psi_{\Delta S^\circ,\mathrm{W}} - \psi_{\Delta S^\circ,\mathrm{R}}$ represent the thermodynamic destabilization caused by mismatched nucleotides. The fitted functions are shown in Fig. S4. By evaluating these functions at $i = 1$, we obtained the averaged values of $\Delta H^\circ$ and $\Delta S^\circ$ for monomers, and thus $\Delta G_{\mathrm{mono,R}}$ and $\Delta G_{\mathrm{mono,W}}$. Thermodynamic parameters for elongated products were then calculated by linearly scaling these values with length using the common slope. The results are summarized in Table S6.

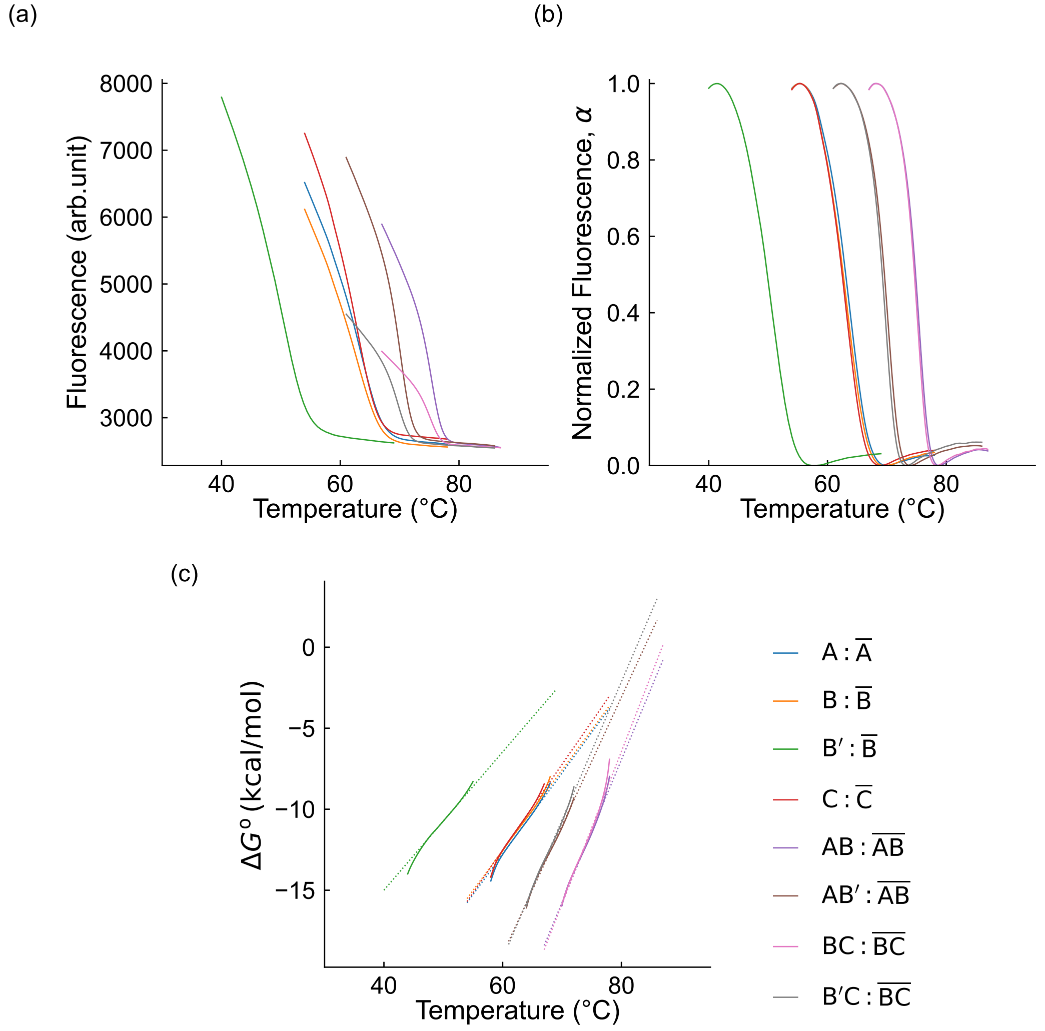


FIG. S3. The melting curves (a) and the normalized melting curves (b), and the obtained standard free energy change (c) associated with hybridization. The dashed lines in (c) are linear fits.

TABLE S6. The thermodynamic parameters obtained by the melting curve analysis.

| Pair | $T_{\mathrm{m}}$ (°C) | $\Delta H^{\mathrm{o}}$ (kcal/mol) | $\Delta S^{\mathrm{o}}$ (cal/mol) | $K_{\mathrm{d}}$ at 66.0 °C (nM) |
|---|---|---|---|---|
| A : $\overline{\mathrm{A}}$ | 64.9 | -177 | -493 | 483 |
| B : $\overline{\mathrm{B}}$ | 64.5 | -180 | -502 | 663 |
| B′ : $\overline{\mathrm{B}}$ | 51.8 | -149 | -427 | 3040000 |
| C : $\overline{\mathrm{C}}$ | 64.1 | -190 | -532 | 977 |
| AB : $\overline{\mathrm{AB}}$ | 75.8 | -319 | -883 | 0.000358 |
| AB′ : $\overline{\mathrm{AB}}$ | 70.6 | -279 | -781 | 0.752 |
| BC : $\overline{\mathrm{BC}}$ | 75.6 | -337 | -936 | 0.000209 |
| B′C : $\overline{\mathrm{BC}}$ | 70.2 | -299 | -840 | 0.828 |
| Correct monomer | 64.5 | -183 ($\Delta H^{\circ}_{\mathrm{mono,R}}$) | -511 ($\Delta S^{\circ}_{\mathrm{mono,R}}$) | 640 |
| Wrong monomer | 52.4 | -147 ($\Delta H^{\circ}_{\mathrm{mono,W}}$) | -419 ($\Delta S^{\circ}_{\mathrm{mono,W}}$) | 1790000 |

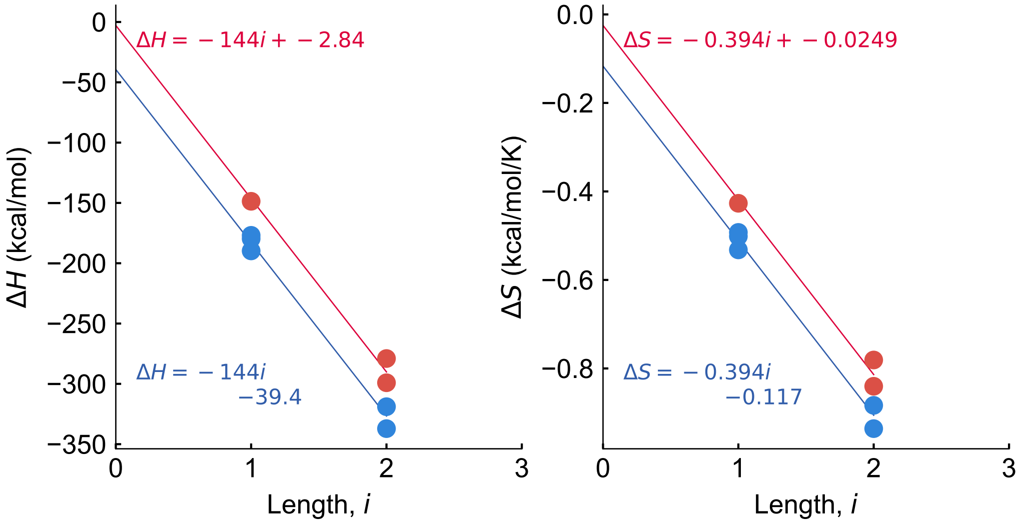


FIG. S4. Length Dependence of $\Delta H$ and $\Delta S$ for the hybridizations with correct pairs (blue) and wrong pairs (red) with linear fits (solid curves). A common slope is used for both fitting conditions.

## S2. SIMULATION

### S2.1. Model

We constructed a model based on ordinary differential equations (ODEs) to simulate the experimental results. The model incorporates three types of reactions: (i) hybridization, (ii) dissociation, and (iii) ligation.

(i) We modeled hybridization as a second-order reaction with an association rate constant $k_{\mathrm{on}}$ assumed to be independent of DNA length. Up to three monomers can bind to the template strand.

(ii) The dissociation rate constant is denoted as $k_{\mathrm{off},i,j}$ where $i$ represents the number of units of a substrate ($1 \leq i \leq l$) that hybridizes to the template with length $l$, and $j$ ($0 \leq j \leq l$) denotes the number of errors in the substrate. The dissociation rate is given by:

$$k_{\mathrm{off},i,j} = k_{\mathrm{on}} K_{\mathrm{d},i,j} = k_{\mathrm{on}} \exp\left[\Delta G_{i,j}/k_{\mathrm{B}} T_{\mathrm{anneal}}\right] \tag{S8}$$

where the Gibbs free energy difference $\Delta G_{i,j}$ is defined as:

$$\Delta G_{i,j} = \Delta G_{\mathrm{mono,R}} + (i-1)\left[\phi_{\Delta H^\circ} + T_{\mathrm{anneal}}\phi_{\Delta S^\circ}\right] + j\Delta\Delta G. \tag{S9}$$

Here, $\Delta\Delta G = \Delta G_{\mathrm{mono,W}} - \Delta G_{\mathrm{mono,R}}$ represents the destabilization due to a single error. The quantities $\Delta G^\circ_{\mathrm{mono,R}}$, $\Delta G^\circ_{\mathrm{mono,W}}$, and the slopes $\phi_{\Delta H^\circ}$, $\phi_{\Delta S^\circ}$ were obtained from the melting curve experiments.

(iii) Ligation occurs with rate constants specific to each combination of DNA strands and their neighboring sequences. The rate constant $k_{\mathrm{L,XY}}$ is chosen based on the terminal unit of the substrates to be ligated. For example, if A and B are ligated, $k_{\mathrm{L,AB}}$ is used, and $k_{\mathrm{L,BC}}$ is used when ligating A'B and C since the mutation A' is not adjacent to the ligation site.

These simplified assumptions allow us to model the reaction dynamics while keeping the number of parameters manageable. For example, consider the dynamics of the complex $\mathrm{A,B}:\overline{\mathrm{ABC}}$ where a colon (:) indicates the hybridized state between substrates (A and B) and the template ($\overline{\mathrm{ABC}}$). An example of the equation is

$$\frac{\mathrm{d}[\mathrm{A,B}:\overline{\mathrm{ABC}}]}{\mathrm{d}t} = k_{\mathrm{on}}[\mathrm{A}:\overline{\mathrm{ABC}}][\mathrm{B}] + k_{\mathrm{on}}[\mathrm{A}][\mathrm{B}:\overline{\mathrm{ABC}}] + k_{\mathrm{off},1,0}[\mathrm{A,B,C}:\overline{\mathrm{ABC}}] \tag{S10}$$

$$-k_{\mathrm{on}}[\mathrm{A,B}:\overline{\mathrm{ABC}}][\mathrm{C}] - 2k_{\mathrm{off},1,0}[\mathrm{A,B}:\overline{\mathrm{ABC}}] - k_{\mathrm{L}}[\mathrm{A,B}:\overline{\mathrm{ABC}}]. \tag{S11}$$

### S2.2. Fitting of the dynamics data in experiments by simulation curves

To test the validity of our simulation, we fitted our model to the result of the dynamics measurement.

We defined six fitting parameters $k_{\mathrm{on}}$, $\delta H$, $k_{\mathrm{L,AB}}$, $k'_{\mathrm{L,AB}}$, $k_{\mathrm{L,BC}}$, and $k'_{\mathrm{L,BC}}$. The hybridization rate of $k_{\mathrm{on}}$ is independent of the substrate length. We introduced $\delta H$ as a modification factor of the free energy change associated with the hybridization of $\mathrm{B'} : \overline{\mathrm{B}}$. Basically, we estimated the Gibbs free energy $\Delta G$ of DNA hybridization using temperature-independent thermodynamic parameters $\Delta H^{\circ}$ and $\Delta S^{\circ}$ obtained from the melting curve analysis. However, in the case of the DNA combination, $\mathrm{B'} : \overline{\mathrm{B}}$, the temperature $T_{\mathrm{anneal}} = 66.0$ °C deviates significantly from the melting temperature $T_{\mathrm{m}} = 51.8$ °C. Thus, a modification to $\Delta G^{\circ}$ was necessary to fit the experimental data. The modification factor $\delta H$ is added to the calculated $\Delta G^{\circ}$ at far from the melting temperature. Other four parameters $k_{\mathrm{L,AB}}$, $k'_{\mathrm{L,AB}}$, $k_{\mathrm{L,BC}}$, and $k'_{\mathrm{L,BC}}$ are the ligation rates, which are defined separately for the DNA combinations to be ligated.

We compared the simulation results to the experimental results through a cost function. We numerically integrated the model and sampled the concentrations and the error fractions at corresponding steps. We defined the cost function as

$$C(\{\mu\},\{\sigma\}|p) = \sum_{m}\left[\left(\frac{\mu_{m,a} - f_{m,a}(p)}{\sigma_{m,a}}\right)^2 \left(\frac{\mu_{m,e} - f_{m,e}(p)}{\sigma_{m,e}}\right)^2\right]. \tag{S12}$$

Here, we collectively denote the fitting parameters $k_{\mathrm{on}}$, $\delta H$, $k_{\mathrm{L,AB}}$, $k'_{\mathrm{L,AB}}$, $k_{\mathrm{L,BC}}$, $k'_{\mathrm{L,BC}}$ as $p$. The summation over $m$ is taken over the product of each length. $\mu_{m,a/e}$ and $\sigma_{m,a/e}$ are the averages and standard errors of the total concentration and the error fraction, respectively. $f_{m,a/e}$ are the values obtained by numerically calculating the ODEs. To simulate the thermal cycles in the experiments, we repeated the calculation of the dynamics for a duration of $\tau = 20$ s at $T_{\mathrm{anneal}}$ 150 times. At the end of each cycle, we dissociated all the dsDNAs to initialize the state for the next calculation. After briefly obtaining parameters using the Optimization.jl package of Julia, we modified the parameters by hand.

We obtained $k_{\mathrm{on}} = 9.41 \times 10^{6}\ \mathrm{M^{-1}s^{-1}}$, $\delta H = -3.85\ \mathrm{kcal\,mol^{-1}}$, $k_{\mathrm{L,AB}} = 0.222\ \mathrm{s^{-1}}$, $k_{\mathrm{L,AB'}} = 0.0190\ \mathrm{s^{-1}}$, $k_{\mathrm{L,BC}} = 0.207\ \mathrm{s^{-1}}$, and $k_{\mathrm{L,BC'}} = 0.00184\ \mathrm{s^{-1}}$. We discuss the validity of the obtained parameters below. The value of $k_{\mathrm{on}}$ was in the order of $10^{6}$, which aligns with the experimentally obtained values reported in some previous literature [3, 5–7]. It is difficult to validate the ligation rates based on reference values because the actual concentration of active ligase is not accessible in experiments, and the ligation rate of the Taq DNA ligase with internal mismatches has not been reported for the present experimental condition. Therefore, we discuss the specificity ratio defined by the ligation rate for the correct DNA strands relative to that of the wrong ones. The specificity ratio was $k_{\mathrm{L,AB}}/k'_{\mathrm{L,AB}} = 11.7$ for the 5' side of the ligation site (A+B ligation), and $k_{\mathrm{L,BC}}/k'_{\mathrm{L,BC}} = 113$ for the 3' side of the ligation site (B+C ligation). Both numbers are compatible with the previous literature [8], where an internal mismatch at various positions was tested, and the specificity ratio was at least 8. The specificity ratio for B+C ligation was almost ten times larger than that of A+B ligation. This could be attributed to the nature of ligase that the mismatch at the 3' side has a larger discrimination ability than the mismatch at the 5' side, as was previously reported [9].

Using the obtained parameters, we counted the cumulative number of transitions from the template states that are ready to be ligated (e.g., $[\mathrm{A}, \mathrm{BC} : \overline{\mathrm{ABC}}]$, $[\mathrm{AB}, \mathrm{C} : \overline{\mathrm{ABC}}]$, $[\mathrm{A}, \mathrm{B'C} : \overline{\mathrm{ABC}}]$, $[\mathrm{AB'}, \mathrm{C} : \overline{\mathrm{ABC}}]$). The types of transitions we consider here are the dissociation and the ligation. We counted 4 types of quantities,

$$m_{2,\mathrm{diss}} = \sum_{i=1}^{150}\int_0^{20} k_{\mathrm{off},2,0}\left\{[\mathrm{A},\mathrm{BC}:\overline{\mathrm{ABC}}] + [\mathrm{AB},\mathrm{C}:\overline{\mathrm{ABC}}]\right\}\mathrm{d}t, \tag{S13}$$

$$m'_{2,\mathrm{diss}} = \sum_{i=1}^{150}\int_0^{20} k_{\mathrm{off},2,1}\left\{[\mathrm{A},\mathrm{B'C}:\overline{\mathrm{ABC}}] + [\mathrm{AB'},\mathrm{C}:\overline{\mathrm{ABC}}]\right\}\mathrm{d}t, \tag{S14}$$

$$m_{3,\mathrm{lig}} = \sum_{i=1}^{150}\int_0^{20} \left\{k_{\mathrm{L,AB}}[\mathrm{A},\mathrm{BC}:\overline{\mathrm{ABC}}] + k_{\mathrm{L,BC}}[\mathrm{AB},\mathrm{C}:\overline{\mathrm{ABC}}]\right\}\mathrm{d}t, \tag{S15}$$

$$m'_{3,\mathrm{lig}} = \sum_{i=1}^{150}\int_0^{20} \left\{k_{\mathrm{L,AB'}}[\mathrm{A},\mathrm{B'C}:\overline{\mathrm{ABC}}] + k_{\mathrm{L,B'C}}[\mathrm{AB'},\mathrm{C}:\overline{\mathrm{ABC}}]\right\}\mathrm{d}t, \tag{S16}$$

(S17)

Here, $m_{2,\mathrm{diss}}$ and $m'_{2,\mathrm{diss}}$ are the cumulative number of dissociation reactions of correct and wrong dimers, respectively. Also, $m_{3,\mathrm{lig}}$, $m'_{3,\mathrm{lig}}$ are the cumulative number of ligation reactions of correct and wrong dimers, respectively.

For dissociation, we included the dissociation by the denaturing step at the end of every cycle. We found that $m_{2,\mathrm{diss}}/m_{3,\mathrm{lig}} = 0.27$ and $m'_{2,\mathrm{diss}}/m'_{3,\mathrm{lig}} = 26$, indicating that dissociation more frequently occurs for the wrong sequence than ligation event. This further confirms the cascade-manner replication.

### S2.3. Temperature dependence in the middle error case

We simulated the temperature dependence of the middle error case using our model obtained from the dynamics experiment. For the cascade case $\mathcal{M}_{\rm cas}$, we used the same model as in the dynamics experiment. For $\mathcal{M}_1$ and $\mathcal{M}_2$, we created another model by reducing the number of states from the model of $\mathcal{M}_{\rm cas}$.

We assumed a constant $k_{\rm on}$ across all temperatures, as no significant temperature dependence was reported in previous studies [5]. For simplicity, ligation rates were also assumed to be constant. Thus, we only assumed the temperature dependence of the hybridization stability. Here, we also added $\delta H = -3.85\,\mathrm{kcal/mol}$ to the free energy change associated with the wrong substrates. With these assumptions, the simulations reproduced the trend in experiments well [see Fig. 3a].

We compared the product $\varepsilon_1\varepsilon_2$ to the observed cascade error fraction, $\varepsilon_{\rm cas}$ [Fig. S5a]. Although there is a slight deviation in absolute values, the similarity between the two quantities suggests that $\varepsilon_{\rm cas}$ can be reasonably approximated by $\varepsilon_1\varepsilon_2$. This trend indicates that the concentration bias established in the first replication stage is effectively propagated to the second stage.

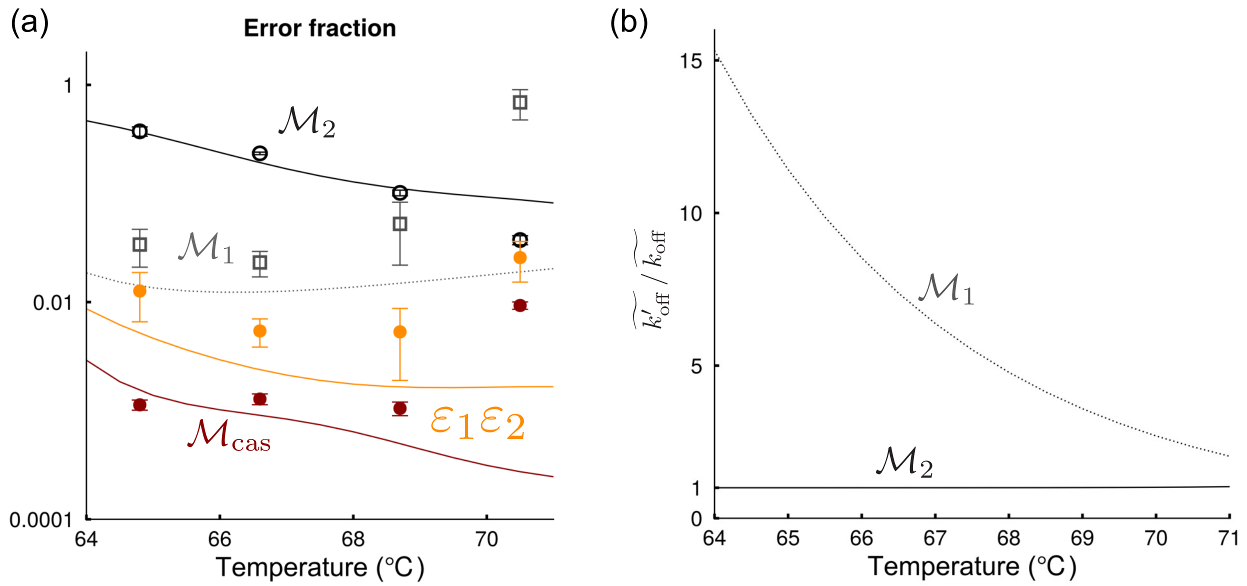


FIG. S5. (a) Temperature dependence of the error fraction when a wrong substrate B′ is incorporated in the middle of the template. Error bars represent standard errors. Yellow symbols and solid curves indicate the product $\varepsilon_1\varepsilon_2$, which closely approximates the observed error fraction in cascade replication, $\varepsilon_{\rm cas}$. Error bars for $\varepsilon_1\varepsilon_2$ were calculated by propagating the errors of $\varepsilon_1$ and $\varepsilon_2$. (b) The ratio $\widetilde{k}'_{\rm off}/\widetilde{k}_{\rm off}$ is calculated for various temperatures. We found $\widetilde{k}'_{\rm off}/\widetilde{k}_{\rm off} \sim 7$ for $\mathcal{M}_1$, which indicates that the dissociation of the wrong monomer more frequently occurs than that of the correct monomer. We also found $\widetilde{k}'_{\rm off}/\widetilde{k}_{\rm off} \sim 1$ for wrong dimers. Together with the ratio $k'_{\rm L}/k_{\rm L}$, $f$ becomes larger than one for both $\mathcal{M}_1$ and $\mathcal{M}_2$, indicating significant error suppression.

## S2.4. Fitting of the temperature dependence of the terminal error case

Similar to the middle error case, we also created models for $\mathcal{T}_{\rm cas}$, $\mathcal{T}_1$ ,$\mathcal{T}_2$, and fitted them to our experimental results [Fig. 3b]. Basically, $k_{\rm on}$, $\delta H$, $k_{\rm L,AB}$, $k_{\rm L,BC}$ are the same to the middle error case. The ligation rate $k_{\rm L,A'B}$, which has not been obtained so fa, was estimated to be $k_{\rm L,A'B} = 5.51 \times 10^{-4}$ by manual fitting. This value is much smaller than $k_{\rm L,AB'}$ and $k_{\rm L,B'C}$. This reduction is not surprising since the number of bases for hybridization of A : A′ is 17, which is a base smaller than B : B′. Moreover, as previously noted, the specificity ratio increases when the error is positioned at the 3' side of the ligation site [9].

We found that the product $\varepsilon_1\varepsilon_2$ and $\varepsilon_{\rm cas}$ have a similar trend with a slight deviation in the absolute values [Fig. S6].

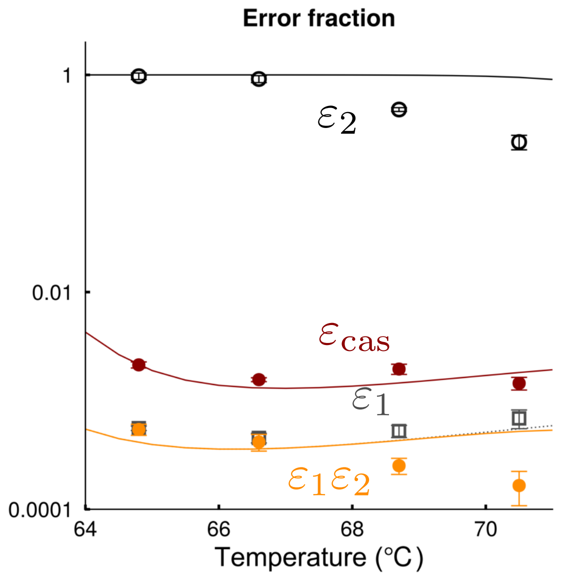


FIG. S6. Temperature dependence of the error fraction when the error is introduced at the terminal position of the template. Error bars represent standard error. The yellow points and line denote the expected error fraction based on the multiplication $\varepsilon_1\varepsilon_2$, which approximates the measured cascade error fraction, $\varepsilon_{\rm cas}$. Same as Fig. S5, error bars in $\varepsilon_1\varepsilon_2$ was estimated by propagating the standard errors of $\varepsilon_1$ and $\varepsilon_2$.

### S2.5. Replication fidelity of longer templates with a single-site error

Here, we describe how the error fraction was calculated for the replication of sequences with length $l \geq 2$, where $l$ denotes the length of the template strand. We focus on the single-site error scenario, where a wrong monomer is incorporated at a specific position within the template [Fig. S7]. The potential error site was fixed at position $\lfloor l/2 \rfloor$, where $\lfloor \cdot \rfloor$ denotes the floor function; for instance, the second for $l = 3$ and 4 and the third for $l = 5$ and 6.

To explore the influence of replication mechanisms on error rates, we simulated two distinct replication modes. The first was the cascade ligation mode, where both hybridization and dissociation processes were modeled for all monomers and intermediates. This setup allows the dissociation and re-binding during the simulation, representing a cascade-like assembly process [Fig. S7a]. The second mode was chain-growth polymerization, in which we set $k_{\mathrm{off},i,j} = 0$ for $i \geq 2$, allowing only monomer hybridization and dissociation while preventing intermediate dissociation [Fig. S7b].

All simulations were conducted using parameter sets that are modified from those used to reproduce experimental results, as the goal of this analysis was not to reproduce specific experimental outcomes but rather to conceptually and visually demonstrate the effectiveness of the error suppression mechanism. Specifically, we examined two cases: one with high hybridization stability ($\Delta G_{\mathrm{mono,R}} = -10\,k_{\mathrm{B}}T$) and another with low hybridization stability ($\Delta G_{\mathrm{mono,R}} = -5\,k_{\mathrm{B}}T$). In both scenarios, the destabilization due to an error was set to $\Delta\Delta G = 1\,k_{\mathrm{B}}T$, as shown in the main text. The template concentration was fixed at 1 nM and the total substrate concentration at each binding domain was set to 40 nM. To maintain this total, we mixed 20 nM of the correct monomer with 20 nM of the wrong monomer. The hybridization rate $k_{\mathrm{on}}$ was set to $10^7$ M/s. For simplicity, the ligation rate was fixed at $k_{\mathrm{L}} = 10\,\mathrm{s}^{-1}$, across all cases, regardless of whether an error was present, its position, or the length of the substrate. Additionally, simulations were performed without implementing thermal cycling. We stopped the simulations when the total concentration of final products, including both correct and wrong sequences, reached a specific threshold. The threshold value was set differently depending on the hybridization stability. Simulations were stopped at 0.1 aM for the low stability case ($\Delta G_{\mathrm{mono,R}} = -5\,k_{\mathrm{B}}T$) and at 1 pM for the high stability case ($\Delta G_{\mathrm{mono,R}} = -10\,k_{\mathrm{B}}T$). The error fraction for sequences of length $l$ was calculated by $\varepsilon(l) = w_l/r_l$ where $r_l$ and $w_l$ are the concentrations of the correct and wrong final products, respectively.

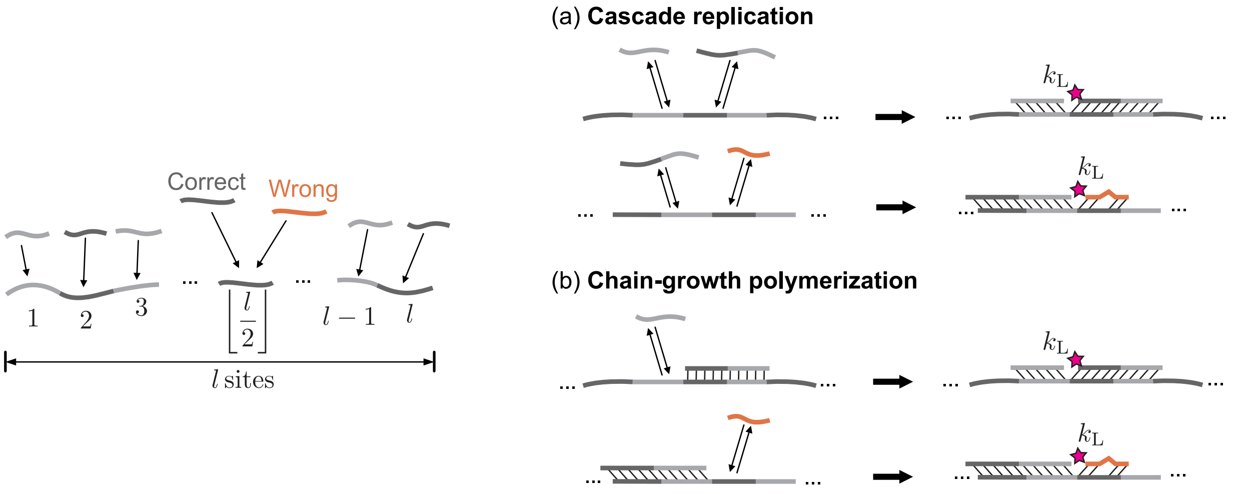


FIG. S7. Replication of a template with length $l$, where an error may be incorporated at a single specific position. (a) Cascade replication, where hybridization and dissociation can occur to all substrates, regardless of their length. (b) Chain-growth polymerization, where only monomers can hybridize to or dissociate from the template.

### S2.6. Replication fidelity of long templates with site-wide error possibility

We extended our model to the cases in which errors may occur at every site of the template [Fig. S8]. Aside from this change, we used the same setup as in the single-site error simulations, including both ligation and chain-growth polymerization modes and the same parameter sets. In this scenario, up to $2^l$ distinct product species can be formed for a template of length $l$, among which only one corresponds to the perfectly replicated product. We quantified the success probability as the concentration ratio of the correct product to the total concentration of all $2^l$ possible products.

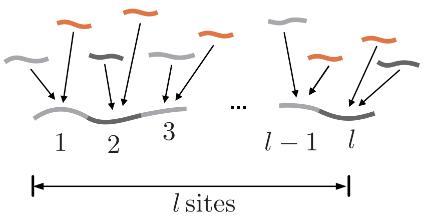


FIG. S8. Replication of long templates with site-wide error possibility. An error might be incorporated at every site on the template.

[1] P. Yaroshchyk and J. E. Eberhardt, Automatic correction of continuum background in laser-induced breakdown spectroscopy using a model-free algorithm, Spectrochim. Acta B **99**, 138 (2014).
[2] G. J. Boggy and P. J. Woolf, A mechanistic model of PCR for accurate quantification of quantitative PCR data, PLOS One **5**, e12355 (2010).
[3] H. Aoyanagi, S. Pigolotti, S. Ono, and S. Toyabe, Error-suppression mechanism of PCR by blocker strands, Biophys. J. **122**, 1334 (2023).
[4] R. Palais and C. T. Wittwer, Mathematical algorithms for high-resolution DNA melting analysis, in *Methods in Enzymology*, Computer Methods, Part A, Vol. 454 (Academic Press, 2009) pp. 323–343.
[5] J. X. Zhang, J. Z. Fang, W. Duan, L. R. Wu, A. W. Zhang, N. Dalchau, B. Yordanov, R. Petersen, A. Phillips, and D. Y. Zhang, Predicting DNA hybridization kinetics from sequence, Nat. Chem. **10**, 91 (2018).
[6] M. Weitz, J. Kim, K. Kapsner, E. Winfree, E. Franco, and F. C. Simmel, Diversity in the dynamical behaviour of a compartmentalized programmable biochemical oscillator, Nat. Chem. **6**, 295 (2014).
[7] B. Yurke and A. P. Mills, Using DNA to power nanostructures, Genet. Program. Evolvable Mach. **4**, 111 (2003).
[8] C. E. Pritchard and E. M. Southern, Effects of base mismatches on joining of short oligodeoxynucleotides by DNA ligases, Nucleic Acids Res. **25**, 3403 (1997).
[9] J. Luo, D. E. Bergstrom, and F. Barany, Improving the fidelity of thermus thermophilus DNA ligase, Nucleic Acids Res. **24**, 3071 (1996).
